# Supplementary material for: Learning Symmetric Rules with SATNet
Source: arXiv:2206.13998 source file (2022-11-25)
Supplement: Supplementary file 1 [file appendix-transfer.tex]

\section{Transfer Learning}

\begin{figure}
    \begin{subfigure}{0.48\columnwidth}
    \includegraphics[width=0.95\linewidth]{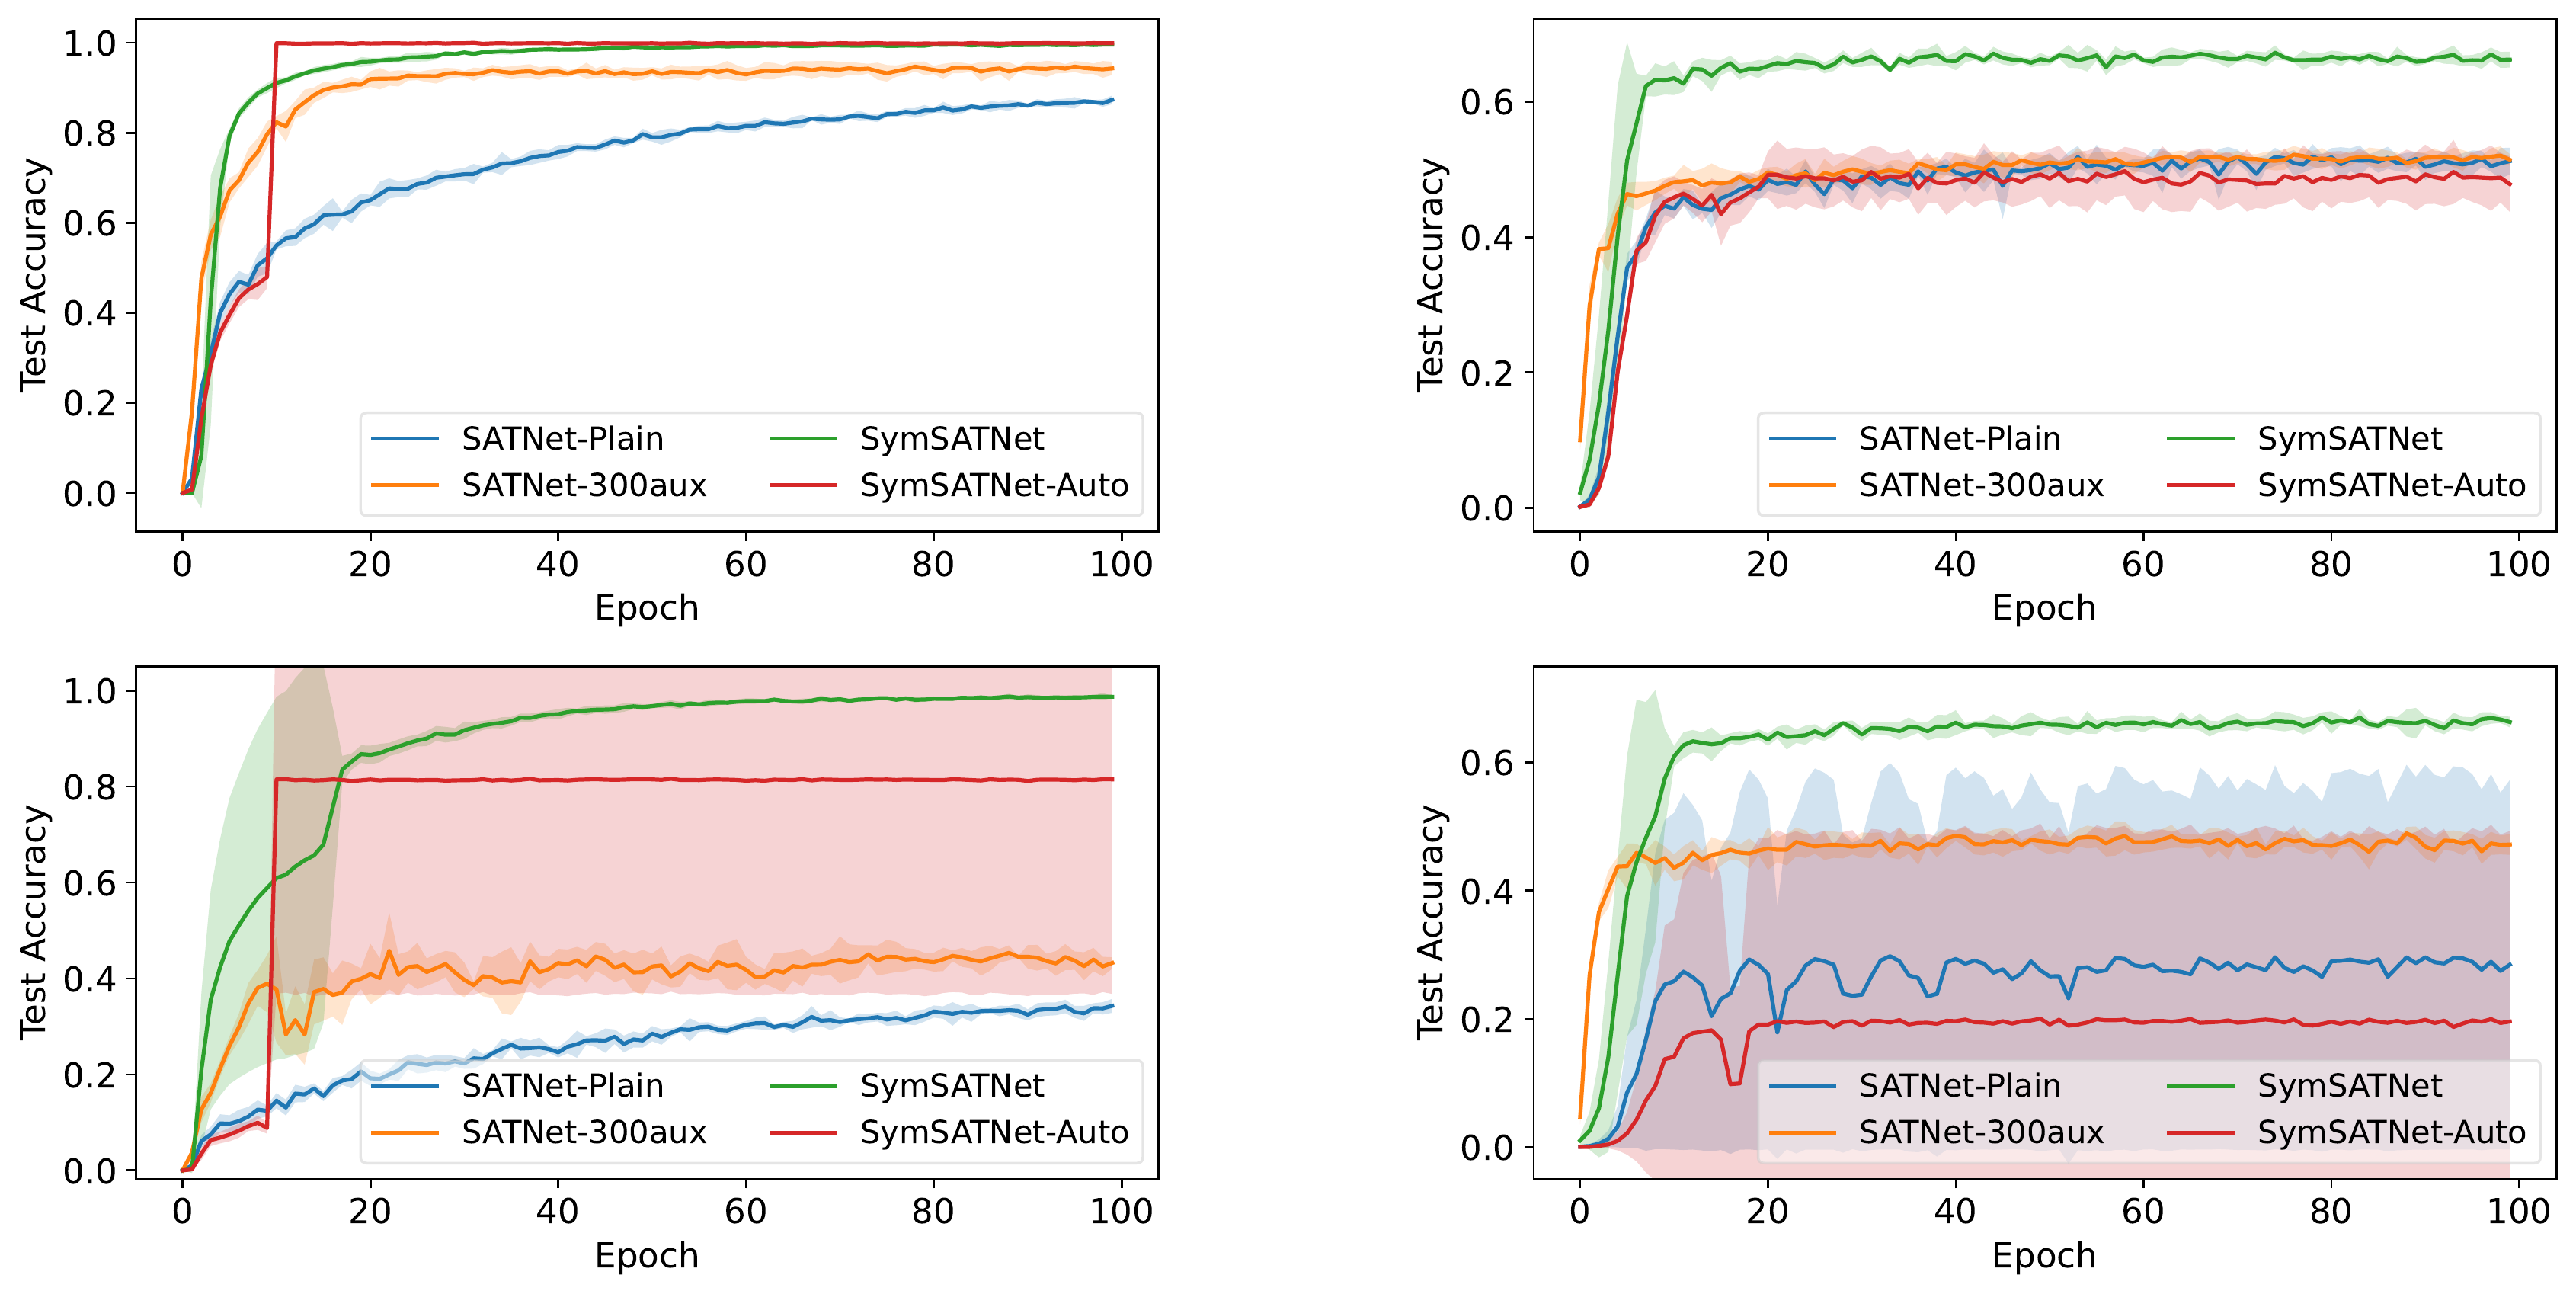}
    \subcaption{Normal Sudoku $\rightarrow$ Hard Sudoku}
    \label{fig:transfer-sudoku-1}
    \end{subfigure}
    \begin{subfigure}{0.48\columnwidth}
    \includegraphics[width=0.94\linewidth]{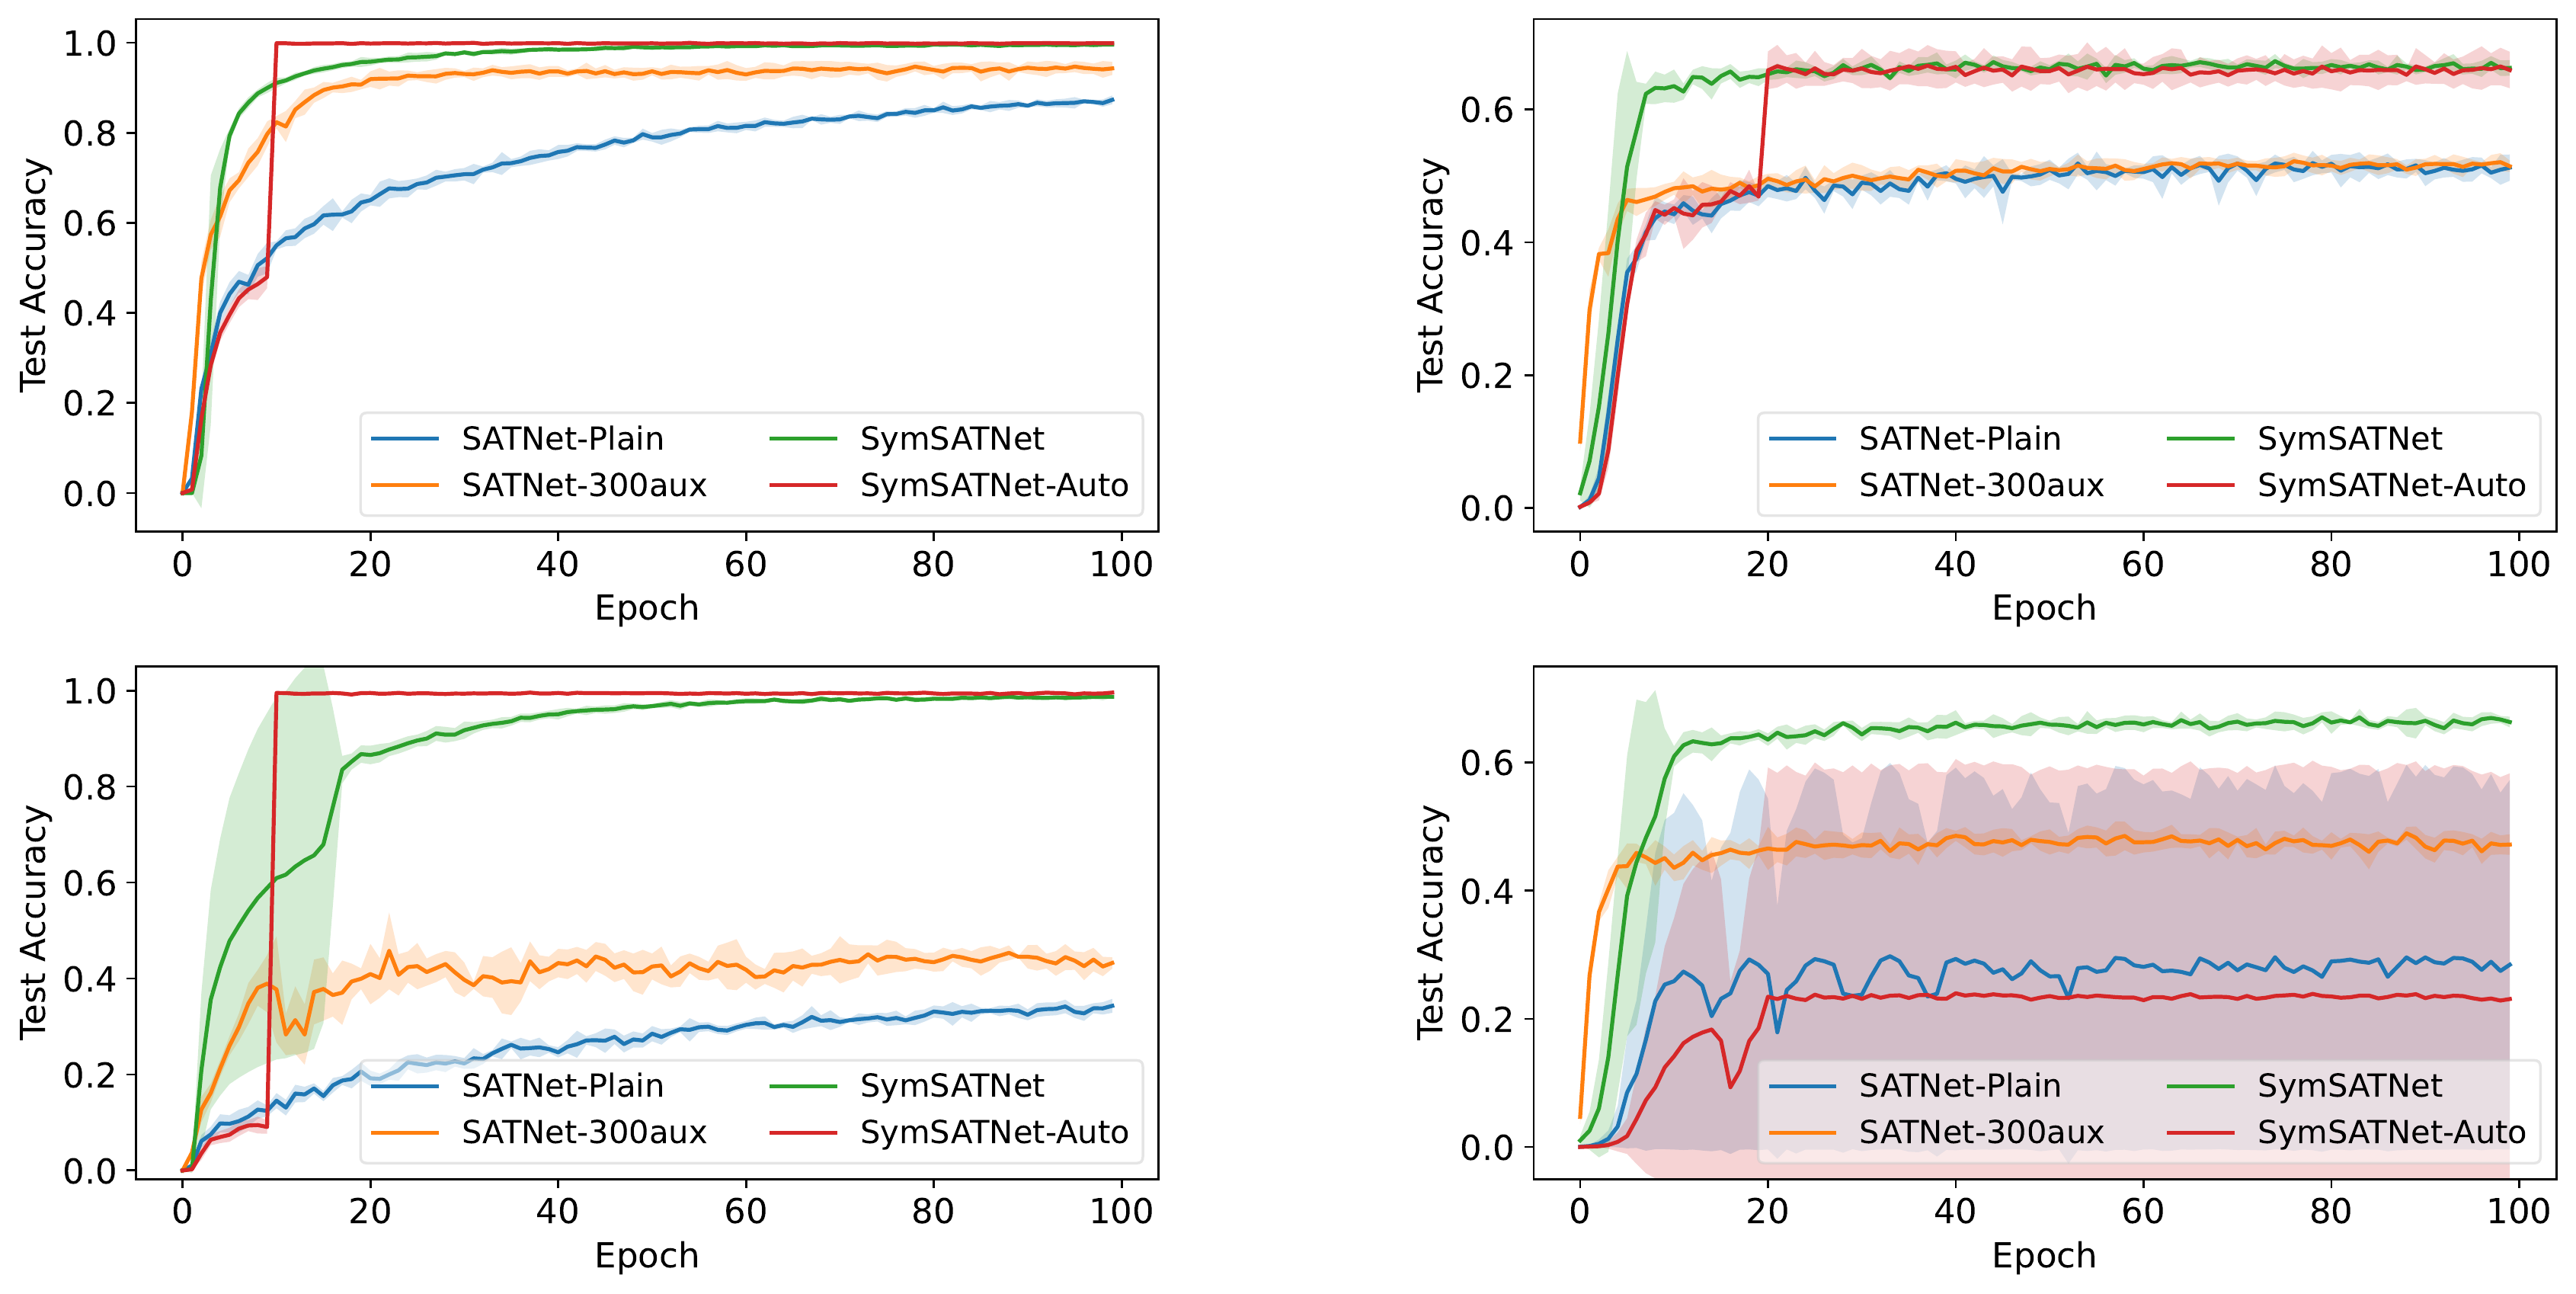}
    \vskip -0.1em
    \subcaption{Normal Rubik's cube $\rightarrow$ Hard Rubik's cube}
    \label{fig:transfer-cube-1}
    \end{subfigure}
    \begin{subfigure}{0.48\columnwidth}
    \includegraphics[width=0.96\linewidth]{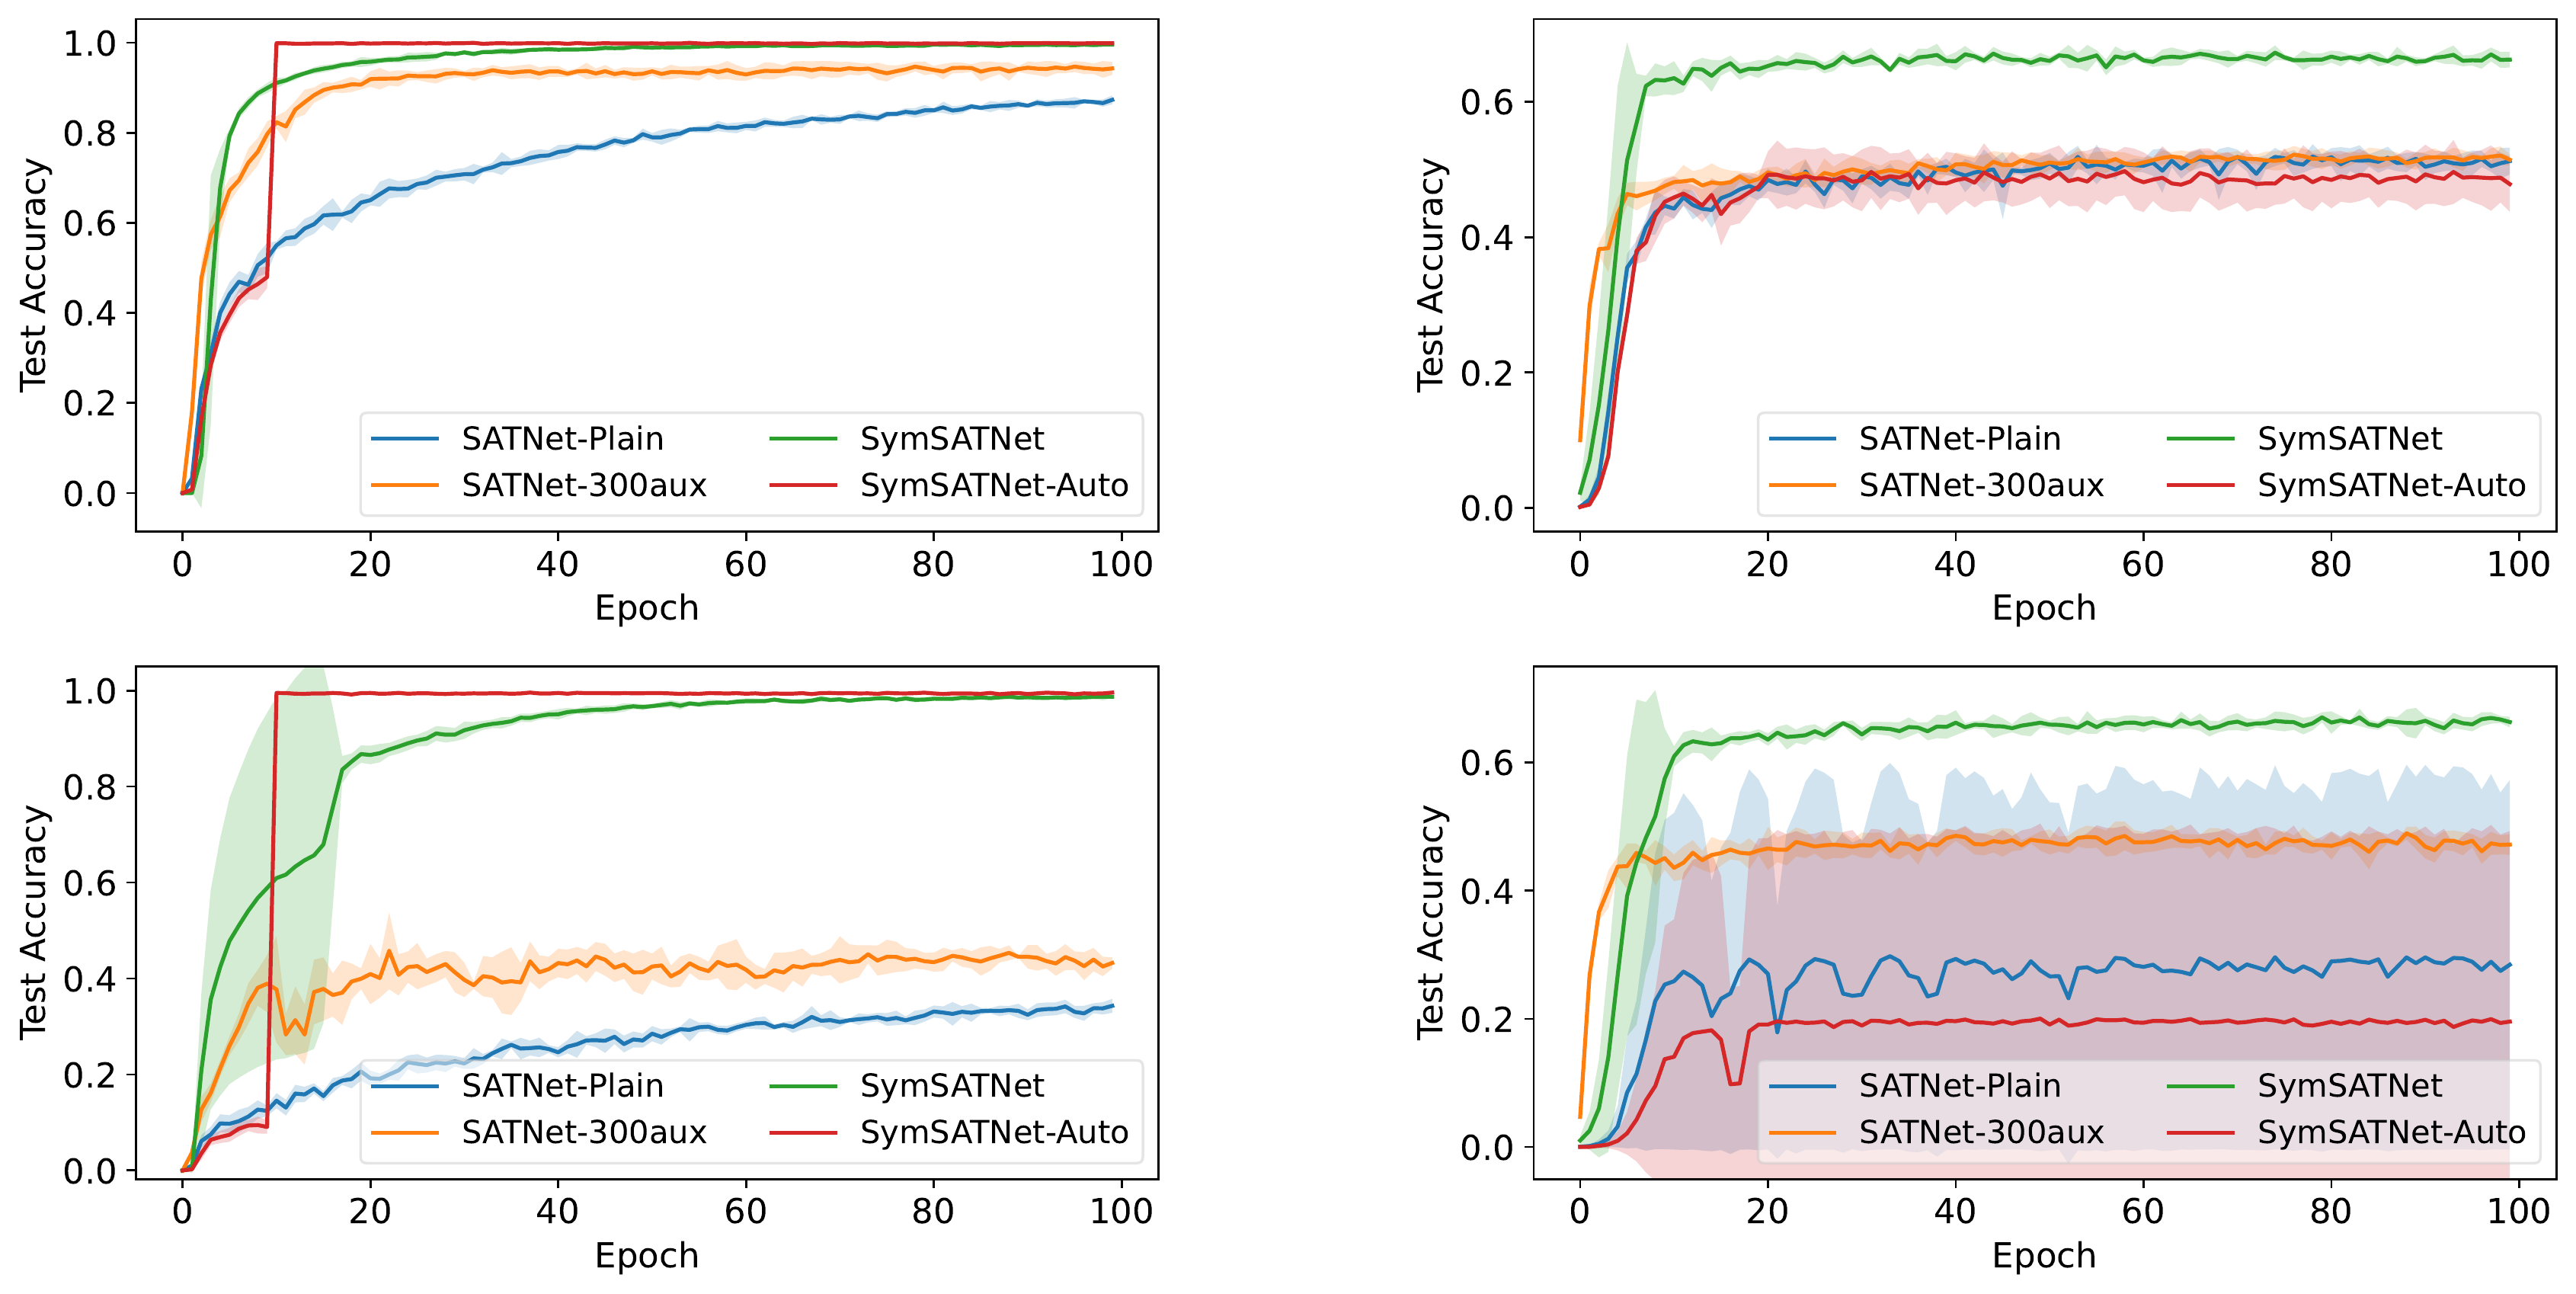}
    \subcaption{Easy Sudoku $\rightarrow$ Hard Sudoku}
    \label{fig:transfer-sudoku-2}
    \end{subfigure}
    \hskip 1.2em
    \begin{subfigure}{0.48\columnwidth}
    \vskip 0.1em
    \includegraphics[width=0.94\linewidth]{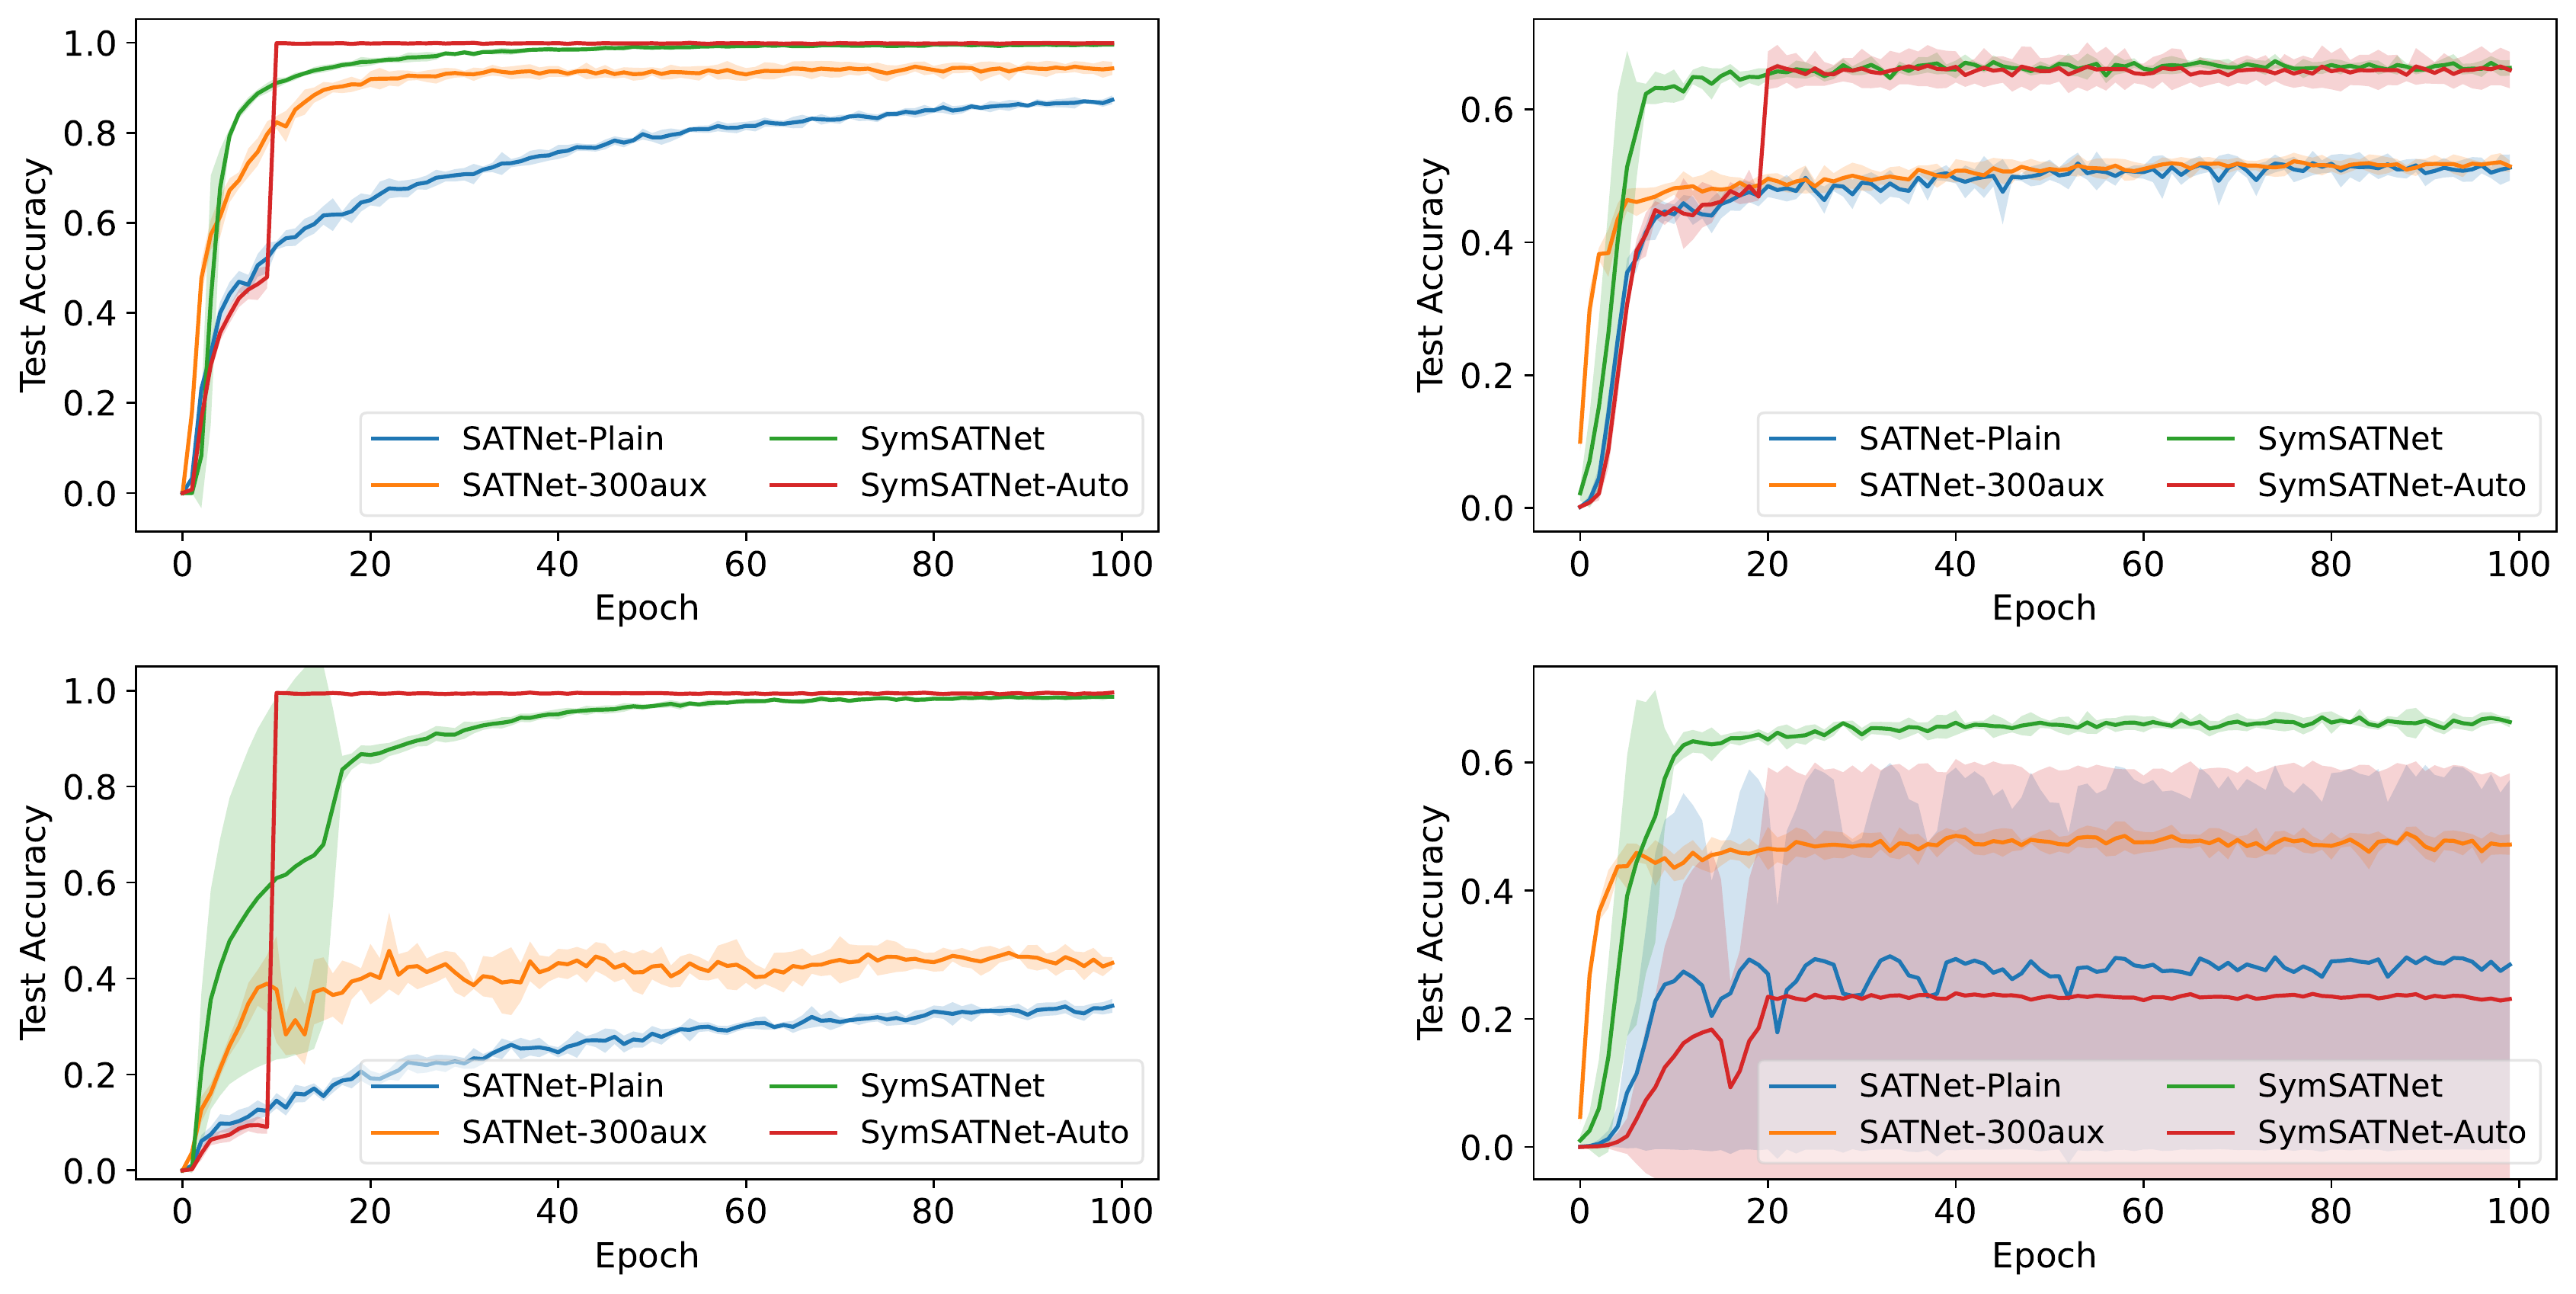}
    \vskip -0.1em
    \subcaption{Easy Rubik's cube $\rightarrow$ Hard Rubik's cube}
    \label{fig:transfer-cube-2}
    \end{subfigure}
    \caption{Transfer learning with various difficulties of training and test examples.
    For both problems, normal and easy examples were used to train, and hard examples were used to train each model.
    Each run was repeated 5 times to report the average test accuracies and $95\%$ confidence interval.}
    \label{fig:transfer}
\end{figure}

\tcb{
To test the transferability of SymSATNet, we generated Sudoku and Rubik's cube examples with various difficulties,
and separated them to build each training dataset with 9K instances of the same difficulties, and each test dataset with 1K instances of the same difficulties.
For SymSATNet-Auto, we split 9K instances in each training dataset into 8K training examples and 1K validation examples.
We used three levels of difficulties of Sudoku and Rubik's cube (easy, normal, hard), each of which determines the number of missing cells for Sudoku or missing facelets for Rubik's cube.
Each input instance of Sudoku was generated with 21 masked cells (easy), or 31 masked cells (normal), or 41 masked cells (hard).
Also, each input instance of Rubik's cube was generated with 3 missing facelets (easy), or 4 missing facelets (normal), or 5 missing facelets (hard).
To guarantee the uniqueness of the solution of the Rubik's cube problem, the number of missing corner facelets, edge facelets, and center facelets did not exceed 2, 2, and 1, respectively.
For both problems, each of normal and easy datasets was used for the training, and hard datasets were used for the test.
We repeated 5 times for each transfer learning task, and reported the average test accuracies and $95\%$ confidence interval.
}

\tcb{
Figure~\ref{fig:transfer} shows the test accuracies through 100 epochs in the four types of transfer learning tasks.
As the results, SymSATNet achieved the best transferabilities in the whole tasks; it succeeded solving the harder problems by applying the rules learnt from much easier training examples.
Also, as Figure~\ref{fig:transfer-sudoku-1},~\ref{fig:transfer-sudoku-2} show, SymSATNet-Auto always exploited the full group symmetries in Sudoku, as it did in our main experiments.
For Rubik's cube, Figure~\ref{fig:transfer-cube-1} shows that SymSATNet-Auto achieved better performance over the baselines by finding partial symmetries as before, when using the normal Rubik's cube dataset.
In contrast, the two baselines in both problems showed their limitation in transfer learning, especially under the big difference of difficulties between training and test examples.
These results show promising abilities of SymSATNet and SymSATNet-Auto to transfer the learnt logical rules from the easier examples to harder instances of problems.
However, for the easy Rubik's cube dataset, SymSATNet-Auto showed poor performance as Figure~\ref{fig:transfer-cube-2} shows.
The main challenge here is due to the violation of the assumption of $\symfind$, that the soft group symmetries of the problem should be learnt by the original SATNet.
In three out of 5 runs to train SymSATNet-Auto with easy Rubik's cube dataset,
SATNet learnt nothing (while producing $0$ accuracies) in the early period of training,
and $\symfind$ returned the trivial group which equated SymSATNet-Auto with SATNet-Plain.
In another two runs, SATNet learnt properly, and $\symfind$ and the validation step found correct partial symmetries, which brought improvement of performance as before.
These results exhibit the fundamental limitation of SymSATNet-Auto using $\symfind$, which strongly depends on the learning performance of the original SATNet.
}
